# Supplementary material for: Designing a Virtual Reality Training Apprenticeship for Cold Spray Advanced Manufacturing
Source: arXiv:2411.08859 source file (2024-11-13)
Supplement: Supplementary file 1 [file Appendix.tex]

\section{Appendix}

\subsection{Pre VR Survey}
The questionnaires included in this survey are \textit{Knowledge Assessment} and \textit{Knowledge Open Response}.

\textbf{Knowledge Assessment}
\begin{enumerate}
    \item Why does bottom wavy spring orientation matter in terms of maintenance?
    \item Why is a light test necessary between the drum and metering block for spray quality?
    \item When putting back bolts into the powder feeder, which tightening pattern should be used for safety?
    \item What is the most vital information to check before dismantling the powder feeder lid to ensure safety?
    \item Why shouldn't the powder feeder-gas hose connections be tightened too much for safety and spray quality?
\end{enumerate}

\textbf{Knowledge Open Questions}
\begin{enumerate}
    \item Provide a list of the Powder Feeder parts' names in their correct assembly order.
    \item Provide the step-by-step procedure for dismantling the powder feeder in the correct order.
\end{enumerate}

\subsection{Post VR Survey}
The questionnaires included in this survey are \textit{Knowledge Assessment}(same as before),\textit{Knowledge Open Responses}(same as before), \textit{VR Insight Open Response}, \textit{NASA-TLX}, \textit{Usability}, and \textit{Presence}.

\textbf{VR Insight Open Response}
These gather user insights relevant to the VRTA itself, the themes that the questions are addressing have been listed along side the the questions in bold. 
\begin{enumerate}
    \item \textbf{[Preparedness]} After playing the VR training, how prepared do you feel to work on the actual powder feeder? Explain why. 
    \item \textbf{[Realism]} How realistic did you find the VR training? Explain why. 
    \item \textbf{[Features]} What parts of the VR training were helpful?
    \item \textbf{[Features]} What parts of the VR training were unhelpful?
    \item \textbf{[Continued VR training]} Would you use this VR training simulation to learn more about Cold Spray? Explain why. 
    \item \textbf{[Additional training]} What other training would you like to take for learning about the powder feeder?
\end{enumerate}

\textbf{NASA-TLX}
The NASA Task Load Index is a multi dimensional rating procedure that provides an overall workload score based on weight average of ratings on six subscales : Mental Demands, Physical Demands, Temporal Demands, Own Performance, Effort and Frustration. This questionnaire is on a 7 point Likert-scale.

\textit{[Very Low to Very High]}
\begin{itemize}
    \item How mentally demanding was the task? 
    \item How physically demanding was the task? [Very Low to Very High]
    \item How hurried or rushed was the pace of the task? [Very Low to Very High]
    \item How hard did you have to work to accomplish your level of performance? [Very Low to Very High]
    \item How insecure, discouraged, irritated, stressed, and annoyed were you? [Very Low to Very High]
\end{itemize}

[Perfect to Failure]
\begin{itemize}
    \item How successful were you in accomplishing what you were asked to do?
\end{itemize}

\textbf{Sense of Immersion/presence}
A sub-scale from the VRUSE survey that focuses on immersion/presence of users in a VR environment. This questionnaire is on a 5 point Likert-scale. 

\textit{[Strongly Disagree to Strongly Agree]}
\begin{itemize}
    \item I felt a sense of being immersed in the virtual environment 
    \item I did not need to feel immersed in the virtual environment to complete my task. [reverse]  
    \item I got a sense of presence (i.e. being there) 
    \item The quality of the image reduced my feeling of presence 
    \item I thought that the field of view enhanced my sense of presence  
    \item The display resolution reduced my sense of immersion 
    \item I felt isolated and not part of the virtual environment
    \item I had a good sense of scale in the virtual environment  
    \item I often did not know where I was in the virtual environment 
\end{itemize}

\textit{[Very Unsatisfactory to Very Satisfactory]}
\begin{itemize}
    \item Overall I would rate my sense of presence as.
\end{itemize}

\textbf{Overall System Usability}
A sub-scale from the VRUSE survey that focuses on the overall system usability of VR application. This questionnaire is on a 5 point Likert-scale. 

\textit{[Strongly Disagree to Strongly Agree]}
\begin{itemize}
    \item I would be comfortable using this system for long periods 
    \item I did not have a clear idea of how to perform a particular function   
    \item The overall system response time did not affect my performance 
    \item I found it difficult to learn how to use the system  
    \item I felt in control of the system 
    \item The system did not work as expected   
    \item I can see a real benefit in this style of man-machine interface 
    \item I found it difficult to work in 3D 
    \item I enjoyed working with the system 

\end{itemize}

\textit{[Far too little to Far too much]}
\begin{itemize}
    \item Overall I would rate the system usability as.
\end{itemize}

\subsubsection{Post Powder Feeder Survey}
The questionnaires included in this survey are \textit{Powder Feeder Insight Questions}, \textit{Previous Experience Questions} and \textit{Demographic Questions}.

\textbf{Powder Feeder Insight Questions}
These questions gather participant insight on working on the real \textit{Powder Feeder}, the themes that the questions are addressing have been listed along side the the questions in bold. 

\begin{itemize}
    \item \textbf{[Preparedness]} How did the VR training help prepare you for the powder feeder task?
    \item \textbf{[Preparedness]} How did the VR training NOT help prepare you for the powder feeder task? 
    \item \textbf{[Realism]} In what ways is the VR training different from actually working on the powder feeder? 
    \item \textbf{[Features]} What should be included in the VR training to make it more helpful? 
    \item \textbf{[Continued VR training]} Would you (still) use this VR training simulation to learn more about Cold Spray? Explain why. 
    \item \textbf{[Additional training]} After the powder feeder task, what training would you like to take for learning about the powder feeder?
\end{itemize}

\textbf{Previous Experience Questions}
These questions gather previous user experience on relevant topics.

\textit{[Never, one or two times, three to five times, more than five times]}
\begin{itemize}
    \item How many times have you experienced any form of virtual reality (VR) environment?
\end{itemize}

\textit{[Never, Rarely, Sometimes, Often, Frequently]}
\begin{itemize}
    \item How often do you play virtual reality (VR) games?
    \item How often do you play computer/video games?
\end{itemize}

\textbf{Demographics}
These questions gather participant demographic information. 

\begin{itemize}
    \item What is your age in years?
    \item What is your major?
    \item What type of student are you? [Undergrad, Masters, PhD, Other]
    \item What is your gender? [Woman, man, Non Binary, Self-describe, Prefer not to answer]
\end{itemize}

\subsection{Retention Survey}
This survey was distributed via email 2 weeks after the in person session with the participants. The questionnaires included in this survey are \textit{Knowledge Assessment}(same as before), \textit{Knowledge Open Responses}(same as before), and \textit{Retention Insight Questions}.

\textbf{Retention Insight Questions}
These questions are primarily open response questions built to gather qualitative information on what they remember from the user study from 2 weeks ago. The themes that the questions are addressing have been listed along side the the questions in bold. 

\begin{itemize}
    \item \textbf{[Retention]} What is your most vivid memory of the VR training in general?
    \item \textbf{[Retention]} Which part of the assembly task do you remember the most? 
    \item \textbf{[Retention]} Which part of the disassembly task do you remember the most? 
    \item \textbf{[Retention]} What do you think you learned the most from the VR training?
    \item \textbf{[Preparedness]} Do you feel prepared to do the powder feeder task again? Please elaborate on why or why not. 
    \item \textbf{[Preparedness]} Which parts of the assembly training do you feel you need to practice again in VR if you had to do the actual powder feeder task again? 
    \item \textbf{[Preparedness]} Which parts of the disassembly training do you feel you need to practice again in VR if you had to do the actual powder feeder task again? 
    \item \textbf{[Continued VR training]} If you were to learn more about cold spray, would you consider continuing to use this VR training? Please elaborate why or why not.   
    \item \textbf{[Continued VR training]} Would you consider choosing VR training to learn in general? Please elaborate why or why not and what topics you would like to learn using VR. 
\end{itemize}

\begin{itemize}
    \item Why did you participate in this study? Provide your strongest reason to participate below.
    \begin{enumerate}
        \item Because it involved the use of virtual reality (VR)
        \item Because it is about advanced manufacturing/cold spray
        \item Because I like to gain experience in research studies
        \item Because I would get a gift card 
        \item Other
    \end{enumerate}
\end{itemize}
